# Supplementary material for: The Space-Efficient Core of Vadalog
Source: arXiv:1809.05951 source file (2018-09-16)
Supplement: Supplementary file 1 [file appendix-proof-trees.tex]

\section{Proofs for Section~\ref{SEC:PWL}}

\subsection{Preliminary Preparations}

\medskip
\noindent
\paragraph{Unraveling the Chase Graph.} Consider again the chase graph
$\ca{G}^{D,\Sigma} = \tup{V, E, \mu}$ for $D$ and $\Sigma$ and a node
$v \in V$.\footnote{Recall that the nodes of $\ca{G}^{D,\Sigma}$ are
  actually atoms from $\chase{D}{\Sigma}$.} The \emph{unraveling of
  $\ca{G}^{D,\Sigma}$ around $v$} is the directed tree
$\ca{G}^{D,\Sigma}_v \coloneqq \tup{V_v, E_v}$, where
\begin{itemize}
\item $V_v$ is the set of all finite sequences
  \begin{align*}
    \ve{v} \coloneqq v_1v_2\cdots v_n
  \end{align*}
  of nodes from $V$ such that $v_1 = v$ and
  $v_{i + 1} E v_i$ for all $i = 1,\ldots,n-1$. We write
  $\last{\ve{v}}$ for $v_n$.
  \item For $\ve{v} = v_1\cdots v_n$ and $\ve{v}' = v_1\cdots v_n v_{n+1}$
    we have that $\ve{v} E_v \ve{v}'$ iff $v_{n+1} E v_n$.
\end{itemize}
Given a set $\Theta \subseteq V$ of nodes, the
\emph{unraveling of $\ca{G}^{D,\Sigma}$ around $\Theta$} is the directed
node- and edge-labeled forest
$\ca{G}^{D,\Sigma}_\Theta = \tup{V_\Theta,E_\Theta,
  \mu_\Theta}$,
where $V_\Theta \coloneqq \bigcup_{v \in \Theta} V_v$ and
$E_\Theta \coloneqq \bigcup_{v \in \Theta} E_v$. For the definition of the
labeling function $\mu_\Theta$, we need some auxiliary notions first.

A \emph{pseudo-path} in $\ca{G}^{D,\Sigma}_\Theta$ is a sequence of nodes
$\ve{v}_1,\ldots,\ve{v}_n$ over $V_\Theta$ such that, for all
$1 \leq i < n$, one of $\ve{v}_{i} E_\Theta \ve{v}_{i+1}$,
$\ve{v}_{i+1} E_\Theta \ve{v}_{i}$, or $|\ve{v}_i| = |\ve{v}_{i+1}| = 1$
holds. Thus, a pseudo-path in the forest $\ca{G}^{D,\Sigma}_\Theta$ is a path in
$\ca{G}^{D,\Sigma}_\Theta$ where we consider the root nodes of the forest to be
connected. Notice that there is thus a unique shortest pseudo-path
between any of two nodes of~$\ca{G}^{D,\Sigma}_\Theta$.

Let $\ve{v} = v_1\cdots v_n$ and $\ve{w} = w_1\cdots w_m$ be nodes from
$\ca{G}^{D,\Sigma}_\Theta$. Given a term $t$, we say that $\ve{v}$ and $\ve{w}$
are \emph{$t$-connected in $\ca{G}^{D,\Sigma}_\Theta$}, if either 
\begin{enumerate*}[label={(\roman*)}]
\item $t$ is a constant and
  $t \in \adom{\mu(\last{\ve{v}})} \cap
  \adom{\mu(\last{\ve{w}})}$, or
\item $t \in \adom{\mu(\last{\ve{u}})}$ for every $\ve{u}$ that
  lies on the unique shortest pseudo-path between $\ve{v}$ and $\ve{w}$
  in $\ca{G}^{D,\Sigma}_\Theta$.
\end{enumerate*}
Clearly, this relation defines an equivalence relation among the nodes
of $\ca{G}^{D,\Sigma}_\Theta$. We write $[\ve{v}]_t$ for the according equivalence
class of $\ve{v} \in V_v$.\footnote{Formally, we set
  $[\ve{v}]_t \coloneqq \set{\tup{\ve{u}, t} \mid \text{$\ve{u}$ is
      $t$-connected to $\ve{v}$}}$ to ensure that
  $[\ve{v}]_{t} = [\ve{w}]_{t'}$ only if $t = t'$.} Moreover, if $a$ is
a constant, then since $[\ve{v}]_a = [\ve{w}]_a$ for any
$\ve{v},\ve{w} \in V_\Theta$, we identify the class $[\ve{v}]_a$ simply
with $a$. For $[\ve{v}]_t$ with $t$ being a labeled null, we
call $[\ve{v}]_t$ a \emph{labeled null} as well.

Now let $\ve{v} \in V_\Theta$ and assume
$\mu(\last{\ve{v}}) = R(t_1,\ldots,t_k)$. Then we define
\begin{align*}
  \mu_\Theta(\ve{v}) \coloneqq R([\ve{v}]_{t_1},\ldots,[\ve{v}]_{t_k}).
\end{align*}
Moreover, if $\ve{v} E_\Theta \ve{w}$ and
$\mu(\last{\ve{v}}, \last{\ve{w}}) = \tup{\sigma, h}$, we set
\begin{align*}
  \mu_\Theta(\ve{v},\ve{w}) &\coloneqq \tup{\sigma, h^\ast}, \quad \text{where } h^\ast \colon x \longmapsto [\ve{v}]_{h(x)}.
\end{align*}

We write $U(\ca{G}^{D,\Sigma},\Theta)$ for the instance
$\bigcup_{\ve{v} \in V_\Theta} \mu_\Theta(\ve{v})$.  Notice that, since we
identify $[\ve{v}]_a$ with $a$ when $a$ is a constant, this entails that
$R(a_1,\ldots,a_n) \in U(\ca{G}^{D,\Sigma},\Theta)$ for every fact
$R(a_1,\ldots,a_n) \in \ca{G}^{D,\Sigma} \upharpoonright \Theta$. Here,
we denote by $\ca{G}^{D,\Sigma} \upharpoonright \Theta$ the set of all
atoms that lie on some path in $\ca{G}^{D,\Sigma}$ that leads from a
database atom to some atom from $\Theta$.

% \begin{lemma}
%   Let $\Gamma \subseteq \chase{D}{\Sigma}$, and consider the unraveling
%   $\ca{G}^\ast_\Gamma$ around $\Gamma$. Then the function
%   $$h \colon [\ve{v}]_t \longmapsto t$$ 
%   is a homomorphism from $\ca{U}(\ca{G}, \Gamma)$ to
%   $\ca{G} \upharpoonright \Gamma$.
% \end{lemma}
% \begin{proof}
%   Immediate by the construction of $\ca{U}(\ca{G},\Gamma)$.
% \end{proof}

Given $\alpha \in U(\ca{G}^{D,\Sigma},\Theta)$, we denote by
$\preds{\alpha}{\sigma}{h}$ the set of children of $\alpha$ whose edge
from $\alpha$ is labeled $\tup{\sigma, h}$.  Accordingly, we write
$\pred{\alpha}$ for the set of all children of $\alpha$. When using this
notation, we assume that the particular unraveling we are refering to is
clear from context.

\begin{lemma}
\label{lem:nullsnew}
Consider an atom $\alpha \in U(\ca{G}^{D,\Sigma},\Theta)$ and suppose that
$\preds{\alpha}{\sigma}{h} = \set{\beta_1,\ldots,\beta_k}$ for some
$\sigma \in \Sigma$ and some $h$. Then if some labeled null occurs in
$\beta_i$, it either occurs also in $\alpha$, or it does not occur in
the label of any node of $\ca{G}^{{D,\Sigma}}_\Theta$ that is not a descendant
of (the node labeling) $\alpha$.
\end{lemma}
\begin{proof}
  Immediate by the definitions of the equivalence classes $[\ve{v}]_t$
  and the labeling function $\mu_\Theta$.
\end{proof}

Let us finally remark that there is an obvious homomorphism $h_\Theta$
from $\Theta$ to $U(\ca{G}^{D,\Sigma},\Theta)$ defined by
$h_\Theta \colon t \mapsto [v_0]_t$, where $v_0$ is any of the root
nodes. Notice that $h_\Theta$ is well-defined, since $[v_0]_t = [w_0]_t$
for all root nodes $v_0,w_0$ of $\ca{G}_\Theta^{D,\Sigma}$ and all
$t \in \adom{\Theta}$. Notice that $h_\Theta$ is indeed a homomorphism,
since, for $\alpha = R(t_1,\ldots,t_n) \in \Theta$,
$h_\Theta(R(t_1,\ldots,t_n)) = R([\alpha]_{t_1},\ldots,[\alpha]_{t_n})
\in U(\ca{G}^{D,\Sigma}, \Theta)$.

\medskip
\noindent
\paragraph{Blocking, Depth, and Rank.} Consider again the unraveling
$\ca{G}^{D,\Sigma}_\Theta$ around $\Theta$, and let
$\alpha \in U(\ca{G}^{D,\Sigma},\Theta)$ be an atom. Suppose that
$\preds{\alpha}{\sigma}{h} = \set{\beta_1,\ldots,\beta_k}$. We say that
\emph{the application of $\beta_1,\ldots,\beta_k \Ra_{\sigma,h} \alpha$
  is blocked in $\Gamma \subseteq U(\ca{G}^{D,\Sigma},\Theta)$}, if there is a
null in $\alpha$ that occurs in $\Gamma \setminus \set{\alpha}$ and does
not appear in one of $\beta_1,\ldots,\beta_k$. Thus, if the application
of $\beta_1,\ldots,\beta_k \Ra_{\sigma,h} \alpha$ is blocked, we cannot
unfold $\Gamma$ into
$\Gamma' \coloneqq (\Gamma \setminus \set{\alpha}) \cup
\set{\beta_1,\ldots,\beta_k}$.
Notice also that every set $\Gamma$ always has at least one $\alpha$
such that for some $\beta_1,\ldots,\beta_k$, the application of
$\beta_1,\ldots,\beta_k \Ra_{\sigma,h} \alpha$ is not blocked for some
$\sigma \in \Sigma$ and some $h$.

The \emph{depth} of $\alpha$, denoted $\dpth{\alpha}$, is defined
inductively as follows:
{\setlength{\jot}{0pt}
\begin{align*}
  \dpth{\alpha} \coloneqq \max\set{\dpth{\beta} \mid\ &\text{$\beta$ is the label of a} \\ &\text{child node of $\alpha$ in $\ca{G}^{D,\Sigma}_\Theta$}} + 1,
\end{align*}
Notice that $\dpth{\alpha} = 1$ iff $\alpha$ labels a leaf node in
$\ca{G}^{D,\Sigma}_\Theta$. For a set of atoms $\Gamma$, we set
$\dpth{\Gamma} \coloneqq \max\set{\dpth{\alpha} \mid \alpha \in
  \Gamma}$.}

The \emph{rank} of $\alpha$, denoted $\rk{\alpha}$, is defined as
\begin{itemize}
\item $\rk{\alpha} \coloneqq 1$, if $\alpha$ is a leaf node in
  $\ca{G}^{D,\Sigma}_\Theta$;
\item $\rk{\alpha} \coloneqq \sum_{\beta \in \pred{\alpha}} \rk{\beta}$,
  otherwise.
\end{itemize}
For a set of atoms $\Gamma$, we set
$\rk{\Gamma}\coloneqq \sum_{\alpha \in \Gamma}
\rk{\alpha}$.
Intuitively, the rank of an atom gives a measure of how many database
facts are used to derive that atom.

Both the depth and rank of atoms will be used as induction parameters
for the proofs of that section. We remark that these parameters are, of
course, always defined relative to a particular unraveling $\ca{U}$ of
$\ca{G}$. The concrete unraveling of $\ca{G}^{D,\Sigma}$ that they refer to will
always be clear from context in the following, and we adhere to no
particular additional notation to indicate the reference to $\ca{U}$.

\subsection{Proof of Item (1) of  Lemma~\ref{lem:existence-ct}}

As explained in the main body of the paper, the implication from (2) to
(1) ~is straightforward and already follows from
Theorem~\ref{the:proof-trees-qans}. We prove the other direction.

Let $D$ be a database and assume that $\Sigma \in \class{WARD}$. Let
$\ca{G}^{D,\Sigma}$ be the chase graph for $\tup{D,\Sigma}$, and consider the
unraveling $\ca{G}_\Theta^{D,\Sigma}$ of $\ca{G}^{D,\Sigma}$ around some
$\Theta \subseteq \chase{D}{\Sigma}$, where. Let
$\Gamma \subseteq U(\ca{G}^{D,\Sigma},\Theta)$ be a set of atoms. We are going
to prove that there exists a chase tree $\ca{T}$ for $\Gamma$
(w.r.t.~$\ca{G}_\Theta^{D,\Sigma}$) whose node-width is bounded by $m_\Gamma$,
where
\begin{align*}
m_\Gamma \coloneqq f_{\class{WARD}}(\Gamma, \Sigma) = 2 \cdot \max \set{|\Gamma|, \max \set{|\body{\sigma}| : \sigma \in \Sigma}}.
\end{align*}

To this end, we proceed by induction on $\dpth{\Gamma}$.

% Let $\ve{c} \in \cert{q}{D}{\N{\Sigma}}$. Hence, there is a homomorphism
% $h$ such that $h(q) \subseteq \chase{D}{\N{\Sigma}}$ and
% $h(\ve{x}) = \ve{c}$. In the following, for a finite
% $\Gamma \subseteq \chase{D}{\N{\Sigma}}$, we let
% \begin{align*}
% m_\Gamma \coloneqq 2 \cdot \max (\set{|\Gamma|} \cup \set{|\body{\sigma}| : \sigma \in \N{\Sigma}}).
% \end{align*}

% By Lemma~\ref{lem:ptct} it suffices to show that there is a chase tree
% $\ca{T}$ for $\Gamma \coloneqq h(q)$ such that
% $\nwd{\ca{T}} \leq m_\Gamma$.  We proceed to show the existence of
% $\ca{T}$ by induction on $\dpth{\Gamma}$.

Assume first that $\dpth{\Gamma} = 1$. Then $\Gamma$ must consist of a
set of facts $\set{\alpha_1,\ldots,\alpha_k} \subseteq D$, and thus a
trivial chase tree for $\Gamma$ is the tree that has its root labeled
with $\Gamma$. The node-width of that tree is trivially at
most~$m_\Gamma$.

Suppose now that $\dpth{\Gamma} = n + 1$. We perform a subsidiary
induction on the number of atoms in $\Gamma$ that have depth $n + 1$.

Suppose first that there is exactly one atom $\alpha \in \Gamma$ that
has depth $n + 1$. Let $\beta_1,\ldots,\beta_k$ be such that
$\preds{\alpha}{\sigma}{h} = \set{\beta_1,\ldots,\beta_k}$ for some
$\sigma \in \Sigma$ and some homomorphism $h$, and such that the
application of $\beta_1,\ldots,\beta_k \Ra_{\sigma,h} \alpha$ is not
blocked in $\Gamma$. (It is easy to see that such an application cannot
be blocked, since $\alpha$ is of maximal depth.) Since $\Sigma$ is
warded, there is at most one ward $\beta_i$ such that all the nulls contained
in $\alpha$ are also present in $\beta_i$. Moreover, $\beta_i$ does not
share any other nulls with any of the $\beta_j$, for $j \neq i$. In case
such a ward $\beta_i$ exists, we set
$\Gamma' \coloneqq (\Gamma \setminus \set{\alpha}) \cup \set{\beta_i}$
and
$\Gamma'' \coloneqq
\set{\beta_1,\ldots,\beta_{i-1},\beta_{i+1},\ldots,\beta_k}$. Otherwise,
we set $\Gamma' \coloneqq \Gamma \setminus \set{\alpha}$ and
$\Gamma'' \coloneqq \set{\beta_1,\ldots,\beta_k}$. In both cases, we see
that $\set{\Gamma', \Gamma''}$ is a decomposition of $\Gamma$, since the
nulls that do not appear in $\alpha$, yet that appear in some atom among
$\beta_1,\ldots,\beta_k$, are all fresh by
Lemma~\ref{lem:nullsnew}. Moreover, we know that there are no nulls that
are present in $\alpha$, yet not in any of the $\beta_1,\ldots,\beta_k$,
since the application of $\beta_1,\ldots,\beta_k \Ra_{\sigma,h} \alpha$
is not blocked in $\Gamma$.

Notice that we have $\dpth{\Gamma'} \leq n$ and
$\dpth{\Gamma''} \leq n$. Hence, by induction hypothesis, there are
chase trees $\ca{T}'$ and $\ca{T}''$ that are respectively for $\Gamma'$
and $\Gamma''$. We build a chase tree $\ca{T}$ for $\Gamma$ by labeling
its root $v_0$ with $\Gamma$, and declaring that $v_0$ has one child
$v_1$ whose label is $\Gamma' \cup \Gamma''$. Furthermore, $v_1$ has two
children, $v'$ and $v''$, that are respectively labeled with $\Gamma'$
and $\Gamma''$. Notice that $m_{\Gamma'} \leq m_\Gamma$ and that
$m_{\Gamma''} \leq m_\Gamma$. Moreover,
$|\Gamma' \cup \Gamma''| \leq |\Gamma| + \max\set{|\body{\sigma}| :
  \sigma \in \Sigma} \leq m_\Gamma$. Thus, $\ca{T}$ is a chase tree for
$\Gamma$ with the desired bound on the node-width.

The induction step of the subsidiary induction is performed
\emph{mutatis mutandis} as the base case and we thus omit it for
brevity. This finishes the proof of
item (1) of Lemma~\ref{lem:existence-ct} \hfill$\qed$

\subsection{Proof of Item (2) of Lemma~\ref{lem:existence-ct}}

Let $D$ be a database and assume that $\Sigma \in \class{WARD}$. Let
$\ca{G}^{D,\Sigma}$ be the chase graph for $\tup{D,\Sigma}$, and
consider the unraveling $\ca{G}_\Theta^{D,\Sigma}$ of $\ca{G}^{D,\Sigma}$
around some $\Theta \subseteq \chase{D}{\Sigma}$. We are going to write
$\lvl{\alpha}$ for $\lvli{\alpha}{\Sigma}$ in the following, and
$\lvl{\Sigma}$ for $\max\set{\lvli{P}{\Sigma} \mid P \in \sch{\Sigma}}$.

Before proceeding to the proof of
Theorem~\ref{the:proof-trees-qans-pwl-warded}, let us define some
additional technical notions.

\medskip
\noindent
\paragraph{Additional normal form transformations.} We say that a set of
piece-wise linear TGDs ${\Sigma}$ is in \emph{level-wise normal form},
if the following condition is satisfied, for every $\sigma \in \Sigma$:
if the head predicate of $\sigma$ has level $k$, then each of the
predicates occurring in $\body{\sigma}$ has level $k$ or $k-1$.

\begin{lemma}
\label{lem:stratnf}
Every piece-wise linear set of TGDs ${\Sigma}$ can be transformed
into a piece-wise linear $\Sigma^+$ in level-wise normal form such that,
for any CQ $q(\ve{x})$ over $\sch{{\Sigma}}$ and any database $D$
over $\sch{{\Sigma}}$, we have that
$\cert{q}{D}{{\Sigma}} = \cert{q}{D}{\Sigma^+}$.

Moreover, $\lvl{\Sigma^+} \leq \lvl{\Sigma}$, and $\Sigma^+$ can be
obtained from $\Sigma$ by introducing polynomially many fresh
predicates, and by only introducing rules that take the form
$R(\ve{x}) \limpl P(\ve{x})$, where $R$ and $P$ are
relational atoms.
\end{lemma}
\begin{proof}
 Suppose $\Sigma$ is not in level-wise normal form. Then there is a
 $\sigma \in \Sigma$ of the form, say,
 \begin{align*}
   \alpha_1,\ldots,\alpha_m \limpl \psi,
 \end{align*}
 (where the $\alpha_1,\ldots,\alpha_m$ are relational atoms and $\psi$
 is an atom some of whose variables are possibly existentially
 quantified) such that it holds that
 $n_i = \lvli{p}{\Sigma} - \lvli{\alpha_i}{\Sigma} > 1$, where $p$ is
 the predicate of the single atom belonging to $\psi$---let us call
 such a $\sigma$ \emph{bad} in the following. For
 $\alpha_i \coloneqq \alpha_i(\ve{x})$, we add to $\Sigma^+$ the rules
 \begin{align*}
   \alpha_i(\ve{x}) &\limpl \alpha_i^{\sigma, 1}(\ve{x}),\\
   \alpha_i^{\sigma, k}(\ve{x}) &\limpl \alpha_i^{\sigma, k + 1}(\ve{x}), \quad\text{for $k \in [n_i-1]$.}
 \end{align*}
 Here, the predicate of the atoms $\alpha_i^{\sigma, k}(\ve{x})$ are
 all fresh. Notice that
 $\lvli{\alpha_i^{\sigma,k}}{\Sigma^+} = \lvli{\alpha_i}{\Sigma} + k$,
 and thus
 $\lvli{\alpha_i^{\sigma, n_i - 1}}{\Sigma^+} = \lvli{p}{\Sigma} - 1$.
 % It is also easy to check that
 % $\stratumi{p[{\alpha_i^{\sigma,k}}]}{\ca{G}} =
 % \stratumi{p[{\alpha_i}]}{\ca{G}} + k$,
 % for any database $D$ and the associated chase graph $\ca{G}$
 % for $\tup{D,\Sigma}$, and thus also
 % $\stratumi{p[\alpha_i^{\sigma, n_i - 1}]}{\ca{G}} =
 % \stratumi{p}{\ca{G}} - 1$.

 Now we add to $\Sigma^+$ the rule
 \begin{align*}
   \alpha_1^{\sigma, n_1},\ldots,\alpha_m^{\sigma, n_m} \limpl \psi.
 \end{align*}
 Notice that $\lvli{p}{\Sigma^+} = \lvli{p}{\Sigma}$. We do this step
 exhaustively for all bad rules $\sigma \in \Sigma$. Moreover, we add
 to $\Sigma^+$ those rules from $\Sigma$ that are not bad without any
 change.
\end{proof}

In the following, we shall assume that, without loss of generality,
$\Sigma$ is presented to us in level-wise normal form.

\medskip
\noindent
\textbf{Conflict-free Atoms.} The \emph{stratification of $\Sigma$} is a
partition $\tup{\ca{S}_1,\ldots,\ca{S}_{\lvl{\Sigma}}}$ of
$\sch{\Sigma}$ such that, for $P \in \sch{\Sigma}$ we have that
$P \in \ca{S}_k$ iff $\lvli{P}{\Sigma} = k$. We let
$\tup{\Gamma[\ca{S}_1],\ldots,\Gamma[\ca{S}_{\lvl{\Sigma}}]}$ denote the
unique partition of $\Gamma \subseteq U(\ca{G}^{D,\Sigma},\Theta)$ such
that for every $\alpha \in \Gamma$ we have
$\alpha \in \Gamma[\ca{S}_{k}]$ if and only if $k = \lvl{\alpha}$.

Given a set of atoms $\Gamma$, the \emph{join graph} of $\Gamma$ is the
undirected edge-labeled graph $\jg{\Gamma}$ whose set of nodes is
$\Gamma$ and that has an edge between $\alpha$ and $\beta$ labeled with
terms $t_1,\ldots,t_k$ iff
\begin{enumerate*}[label={(\roman*)}]
\item  $\alpha \neq \beta$ and 
\item $t_1,\ldots,t_k$ exhausts all terms that occur in both $\alpha$
  and~$\beta$.
\end{enumerate*}

We say that an atom $\alpha \in \Gamma[\ca{S}_i]$ is \emph{conflict-free
  (in $\Gamma$)}, if there is no atom
$\beta \in \bigcup_{j > i} \Gamma[\ca{S}_j]$ such that there is a path
from $\alpha$ to $\beta$ in $\jg{\Gamma}$ that has an occurrence of a
null in each of its edge labels -- we shall call such a path
\emph{conflicting}. Hence, an atom that only has constants as arguments
is trivially conflict-free. Notice also that every $\Gamma$ trivially
has conflict-free atoms, namely those that are among $\Gamma[\ca{S}_r]$,
where $r$ is the largest number such that $\Gamma[\ca{S}_r]$ is
non-empty.

\medskip
\noindent
\textbf{Size Measures.} For $\Gamma \subseteq U(\ca{G}^{D,\Sigma},\Theta)$, we
let
\begin{align*}
  l_\Gamma \coloneqq \min\set{k \mid \exists \alpha \in \Gamma[\ca{S}_k] \colon \text{$\alpha$ is conflict-free}},
\end{align*}
and we write $b$ for $\max\set{|\body{\sigma}| : \sigma \in
  \Sigma}$. Given $\Gamma$, we let
$$\tup{a^\Gamma_1,\ldots,a_{\lvl{\Sigma}}^\Gamma}\quad \text{ and }\quad \tup{n_1^\Gamma,\ldots,n^\Gamma_{\lvl{\Sigma}}}$$
be sequences of natural numbers such that
$a_i^\Gamma = |\Gamma[\ca{S}_i]|$ and $n_i^\Gamma$ is the number of
atoms from $\Gamma[\ca{S}_i]$ that are \emph{not}
conflict-free. 

We set
\begin{align*}
  m_\Gamma \coloneqq{}& \sum_{i =1}^{\lvl{\Sigma}} b\cdot \max\set{a_i^\Gamma , 1 + n_i^\Gamma}.
\end{align*}

\begin{proof}[Proof of item (2) of Lemma~\ref{lem:existence-ct}]
  Let $\Gamma \subseteq U(\ca{G}^{D,\Sigma},\Theta)$. We are going
  to prove that there exists a chase tree $\ca{T}$ for $\Gamma$
  (w.r.t.~$\ca{G}_\Theta^{D,\Sigma}$) whose node-width is bounded by
  $m_\Gamma$. This suffices to prove the claim, since
  $m_\Gamma \leq f_{\class{WARD} \cap \class{PWL}}(\Gamma, \Sigma)$. To
  this end, we shall proceed by induction on $\rk{\Gamma}$.

\textit{Base case.} Suppose first that $\rk{\Gamma} = 1$. The
\emph{level depth} of $\Gamma$ is
  \begin{align*}
    \ldpth{\Gamma} \coloneqq \max\set{\dpth{\alpha} \mid\ \alpha \in \Gamma[\ca{S}_{l_\Gamma}] \text{ and $\alpha$ is conflict-free}}.
  \end{align*}
  We perform an auxiliary induction on $\ldpth{\Gamma}$ in order to
  prove our claim.
  
  Suppose that $\ldpth{\Gamma} = 1$. Since $\rk{\Gamma} = 1$, this means
  that actually $\Gamma = \set{\alpha}$ for some fact $\alpha \in D$. A
  linear chase tree for $\Gamma$ of node-width at most
  $m_\Gamma \geq |\Gamma|$ is simply the tree with a single root node
  whose label is $\Gamma$.

  Suppose now that $\rk{\Gamma} = 1$ and $\ldpth{\Gamma} = n + 1$. This
  means that $\Gamma = \set{\alpha}$ for some atom $\alpha$ such that
  $\preds{\alpha}{\sigma}{h} = \set{\beta}$ for some atom $\beta$ (and some
  $\sigma \in \Sigma$ and some homomorphism $h$) with
  $\dpth{\beta} = n$. We let $\Gamma' \coloneqq \set{\beta}$, and we
  observe that $\ldpth{\Gamma} = n$. By induction hypothesis, there is a
  linear chase tree $\ca{T}'$ for $\Gamma'$ whose node-width is bounded
  by $m_{\Gamma'}$. Let $\ca{T}$ be the linear chase tree whose root
  $v_0$ is labeled with $\Gamma$, and such that $v_0$ has a single child
  labeled with $\Gamma'$. It is easy to check that
  $m_{\Gamma} = m_{\Gamma'} = b$. Thus, $\ca{T}$ is a linear chase tree for
  $\Gamma$ whose node-width is bounded by $m_\Gamma$, as desired.

  \textit{Induction step.}  Suppose now that $\rk{\Gamma} = m + 1$. A
  \emph{reduction sequence for $\Gamma$} is a finite sequence
  $\tup{\Gamma_0,\Gamma_1,\ldots,\Gamma_k,\Xi}$ of sets of atoms that
  satisfy the following conditions:
  \begin{enumerate}
  \item $\Gamma_0 = \Gamma$, 
  \item $m_{\Gamma_0} \geq m_{\Gamma_1} \geq \cdots \geq m_{\Gamma_k}$,
  \item each $\Gamma_{i+1}$ is an unfolding of $\Gamma_i$, where
    $i = 0,\ldots,k-2$,
  \item $\rk{\Gamma_k} \leq m$, and
  \item $\Xi = \Gamma_{k-1} \cap D$ and
    $\Gamma_{k} = \Gamma_{k-1} \setminus \Xi$. Thus,
    $\set{\Gamma_k, \Xi}$ is a decomposition of $\Gamma_{k-1}$.
  \end{enumerate}

  \begin{lemma}
    \label{lem:redsequence}
    There exists a reduction sequence for $\Gamma$.
  \end{lemma}
  \begin{proof}
  We shall also perform a subsidiary induction on $\ldpth{\Gamma}$ to
  show that, for every $n \geq 1$, if $\ldpth{\Gamma} = n$, then there
  exists a reduction sequence for $\Gamma$.

  So suppose first that $\ldpth{\Gamma} = 1$. This means that $\Gamma$
  contains at least one fact from $D$. Let
  $\set{\alpha_1,\ldots,\alpha_k} = \Gamma \cap D$. We form the
  reduction sequence
  $\pi \coloneqq \tup{\Gamma, \Gamma', \set{\alpha_1,\ldots,\alpha_k}}$,
  where
  $\Gamma' \coloneqq \Gamma \setminus \set{\alpha_1,\ldots,\alpha_k}$.
  Notice that $\rk{\Gamma'} \leq m$. In order to prove that $\pi$ is
  indeed a reduction sequence for $\Gamma$, it remains to be shown that
  $m_{\Gamma'} \leq m_{\Gamma}$. Observe that
  \begin{align*}
     m_{\Gamma} - m_{\Gamma'} ={}&
      \sum_{i = 1}^{\lvl{\Sigma}} b \cdot \max\set{a_i^\Gamma, 1 + n_i^\Gamma} - \sum_{i = 1}^{\lvl{\Sigma}} b \cdot \max\set{a_i^{\Gamma'}, 1 + n_i^{\Gamma'}} \\
     ={}& b \cdot \underbrace{\max\set{a_{l_\Gamma}^\Gamma, 1 + n_{l_\Gamma}^\Gamma}}_{=\, a_{l_\Gamma}^\Gamma \text{ since $k \geq 1$}} -\ b \cdot \max\set{\underbrace{a_{l_\Gamma}^{\Gamma'}}_{=\, a_{l_\Gamma}^\Gamma - k}, \overbrace{1 + n_{l_\Gamma}^{\Gamma'}}^{=\, 1 + n_{l_\Gamma}^\Gamma}}.
  \end{align*}
  Now if $a_{l_\Gamma}^\Gamma - k \geq 1 + n_{l_\Gamma}^\Gamma$, then we
  obtain
  \begin{align*}
    m_\Gamma - m_{\Gamma'} = b a_{l_\Gamma}^\Gamma - b(a_{l_\Gamma}^\Gamma - k) = bk > 0,
  \end{align*}
  and if $a_{l_\Gamma}^\Gamma - k < 1 + n_{l_\Gamma}^\Gamma$ we obtain
  \begin{align*}
     m_\Gamma - m_{\Gamma'} = b a_{l_\Gamma}^\Gamma - b(1 + n_{l_\Gamma}^\Gamma) \geq 0,\quad\text{since $1 + n_{l_\Gamma}^\Gamma \leq a_{l_\Gamma}^\Gamma$.}
  \end{align*}
  Thus, in both cases we have that $m_\Gamma \leq m_{\Gamma'}$.

  Suppose now that $\ldpth{\Gamma} = n + 1$. Let
  $\alpha_1,\ldots,\alpha_k$ enumerate all the conflict-free atoms from
  $\Gamma[\ca{S}_{l_\Gamma}]$ of maximal depth (i.e., $n + 1$). For
  $i = 1,\ldots,k$, we let $\sigma_i \in \Sigma$ and $h_i$ be such that
  $\preds{\alpha_i}{\sigma_i}{h_i} =
  \set{\beta_{i,1},\ldots,\beta_{i,k_i}}$,
  for some $\beta_{i,1},\ldots,\beta_{i,k_i}$ such that the application
  of $\beta_{i,1},\ldots,\beta_{i,k_i} \Ra_{\sigma_i,h_i} \alpha_i$ is
  not blocked in $\Gamma$ -- notice that all these objects exist, since
  each of the $\alpha_i$ is conflict-free in $\Gamma$ and of maximal
  depth.

  Let $\Gamma_0 \coloneqq \Gamma$ and
  $\Gamma_i \coloneqq (\Gamma_{i-1} \setminus \set{\alpha_i}) \cup
  \set{\beta_{i,1},\ldots,\beta_{i,k_i}}$, for all $i = 1,\ldots,k$.
  
  \begin{claim}
  \label{claim:level}
  For $i = 1,\ldots,k$, either $l_{\Gamma_i} = l_{\Gamma_{i-1}}$ or
  $l_{\Gamma_i} = l_{\Gamma_{i-1}} - 1$.
  \end{claim}
  \begin{proof}
    As a preliminary remark, notice that, by our normal form
    assumptions, we know that
    $\lvl{\beta_{i,j}} \in \set{\lvl{\alpha_i}, \lvl{\alpha_i} - 1}$ for
    all $j = 1,\ldots,k_i$.

    % Moreover, since $\Sigma$ is piece-wise
    % linear, at most one of the $\beta_{i,j}$ can have the same level as
    % $\alpha_i$.

    We distinguish cases. Suppose first that $\alpha_i$ has no labeled
    nulls as arguments. In this case, all nulls appearing in
    $\beta_{i,1},\ldots,\beta_{i,k_i}$ must be new in the sense that
    they do not appear in $\Gamma_{i-1}$
    (cf.~Lemma~\ref{lem:nullsnew}). Thus, at least one of
    $\beta_{i,1},\ldots,\beta_{i,k_i}$ must be conflict-free in
    $\Gamma_{i}$ and hence $l_{\Gamma_i} = l_{\Gamma_{i-1}}$ or
    $l_{\Gamma_i} = l_{\Gamma_{i-1}} - 1$, since $\Sigma$ is in
    level-wise normal form. This proves the claim for this case.

    Suppose now that $\alpha_i$ has labeled nulls as arguments. Since
    $\Sigma$ is warded, it must be the case that $\sigma_i$ has at most
    one atom in its body (the ward) that shares nulls with $\alpha_i$ at
    all. Suppose first that $\sigma_i$ has no ward in its body. All
    labeled nulls that appear in $\alpha_i$ are thus not present in
    $\beta_{i,1},\ldots,\beta_{i,k_i}$ (Lemma~\ref{lem:nullsnew}) and,
    moreover, all the nulls that appear in
    $\beta_{i,1},\ldots,\beta_{i,k_i}$ do not appear in $\Gamma_{i-1}$,
    whence it follows that at least one of
    $\beta_{i,1},\ldots,\beta_{i,k_i}$ must be conflict-free in
    $\Gamma_i$.  Hence, $l_{\Gamma_i} = l_{\Gamma_{i-1}}$ or
    $l_{\Gamma_i} = l_{\Gamma_{i-1}} - 1$.

    Suppose now that $\beta_{i,j}$ is the ward among
    $\beta_{i,1},\ldots,\beta_{i,k_i}$. If $k_i \geq 2$, then the claim
    is immediate, since the atoms from
    $\set{\beta_{i,1},\ldots,\beta_{i,k_i}} \setminus \set{\beta_{i,j}}$
    are all conflict-free in $\Gamma_{i}$ due to the fact that the nulls
    they contain do not appear in $\Gamma_{i-1}$ by
    Lemma~\ref{lem:nullsnew}. Suppose now that $k_i = 1$. Then
    $\beta_{i,j}$ is conflict-free in $\Gamma_{i}$ or not. In the former
    case, we immediately obtain $l_{\Gamma_{i}} \leq l_{\Gamma_{i-1}}$
    and thus $l_{\Gamma_i} = l_{\Gamma_{i-1}}$ or
    $l_{\Gamma_i} = l_{\Gamma_{i-1}} - 1$ by our normal form
    assumption. In the latter case, $\beta_{i,j}$ is connected to some
    atom
    $\gamma \in \bigcup_{r > \lvl{\beta_{i,j}}} \Gamma_{i}[\ca{S}_r]$ in
    the join graph of $\Gamma_{i-1}$ via a path that is
    conflicting. Notice again that all the nulls that occur in
    $\beta_{i,j}$ are either only contained in $\beta_{i,j}$ or they
    also appear in $\alpha_i$ (cf.~Lemma~\ref{lem:nullsnew}).  Hence,
    there is also a conflicting path in $\jg{\Gamma_{i-1}}$ that
    connects $\alpha_i$ and $\gamma$. Since $\alpha_i$ was assumed to be
    conflict-free in $\Gamma_{i-1}$, it follows that
    $\gamma \in \Gamma_{i-1}[\ca{S}_1] \cup \cdots \cup
    \Gamma_{i-1}[\ca{S}_{\lvl{\alpha}}]$.  Moreover, this entails that
    $\gamma$ is conflict-free in $\Gamma_{i-1}$. Now $\gamma$ must also
    be conflict-free in $\Gamma_{i}$, since all the nulls present in
    $\Gamma_{i}$ that do not occur in $\Gamma_{i-1}$ must be solely
    contained in $\beta_{i,j}$. Thus,
    $l_{\Gamma_i} \leq l_{\Gamma_{i-1}}$ and so
    $l_{\Gamma_i} = l_{\Gamma_{i-1}}$ or
    $l_{\Gamma_i} = l_{\Gamma_{i-1}} - 1$, since $\Sigma$ is in
    level-wise normal form.
  \end{proof}

  \begin{claim}
    \label{claim:levelsucc}
    Assume that $l_{\Gamma_i} = l_{\Gamma_{i-1}} - 1$ and that
    there is a $\beta_{i,j}$ that is not conflict-free in
    $\Gamma_i$. Then there is a
    $\gamma \in \Gamma_i[\ca{S}_{l_{\Gamma_{i-1}}}]$ that is conflict
    free in $\Gamma_i$.
  \end{claim}
  \begin{proof}
    Notice that $\lvl{\beta_{i,j}} = l_{\Gamma_i}$, since all the nulls
    appearing in $\beta_{i,j}$ either occur also in $\alpha_i$ or are
    fresh. Hence, if we had
    $\lvl{\beta_{i,j}} = l_{\Gamma_{i-1}} = l_{\Gamma_i} + 1$, then
    $\alpha$ would not be conflict-free as well. Now since $\beta_{i,j}$
    is not conflict-free, it follows that $\beta_{i,j}$ is connected via
    a conflicting path to some
    $\gamma \in \bigcup_{r > \lvl{\beta_{i,j}}} \Gamma_i[\ca{S}_r]$. It
    is easy to see that, in fact, we must have
    $\lvl{\gamma} = \lvl{\beta_{i,j}} + 1 = l_{\Gamma_{i-1}}$. Now
    $\beta_{i,j}$ therefore shares a null with $\gamma$, and thus
    $\gamma$ shares a null with $\alpha_i$. Hence, $\gamma$ must be
    conflict-free since $\alpha_i$ is.
  \end{proof}

  \begin{claim}
    \label{claim:levelsameandone}
    Suppose that $l_{\Gamma_i} = l_{\Gamma_{i-1}} = 1$. Then $k_i = 1$.
  \end{claim}
  \begin{proof}
    Since $\ldpth{\alpha_i} = n + 1 \geq 2$, $\lvl{\alpha_i} = 1$ only
    if $\alpha_i$ is derived by a sequence of atoms that have the same
    predicate as $\alpha_i$. Hence, we must necessarily have $k_i = 1$,
    since $\Sigma$ is piece-wise linear.
  \end{proof}

  \begin{claim}
    \label{claim:levelsame}
    Assume that $l =l_{\Gamma_i} = l_{\Gamma_{i-1}} > 1$. Then
    $|\Gamma_i[\ca{S}_{l}] \setminus \Gamma_{i-1}[\ca{S}_{l-1}]| \leq
    1$, i.e., $a_{l-1}^{\Gamma_i} - a_{l-1}^{\Gamma_{i-1}} \leq 1$.
  \end{claim}
  \begin{proof}
    Suppose $a_{l-1}^{\Gamma_i} - a_{l-1}^{\Gamma_{i-1}} > 1$, i.e., at
    least two of the $\beta_{i,1},\ldots,\beta_{i,k_i}$ have level
    $l - 1$. Since $l_{\Gamma_i} = l_{\Gamma_{i-1}}$, this means that
    they are actually not conflict-free, whence it follows that they
    share a null with $\alpha_i$. But this is impossible, since at most
    one of the $\beta_{i,1},\ldots,\beta_{i,k_i}$ can share nulls with
    $\alpha_i$ by wardedness.
  \end{proof}

  \begin{claim}
    \label{claim:main-claim-pwl}
    For $i = 1,\ldots,k$, it holds that
    $m_{\Gamma_i} \leq m_{\Gamma_{i-1}}$.
  \end{claim}
  \begin{proof}
    For the sake of readability, let us set
    $l \coloneqq l_{\Gamma_{i-1}}$, $l' = l_{\Gamma_i}$,
    $\Gamma \coloneqq \Gamma_{i-1}$, and $\Gamma' \coloneqq \Gamma_i$ in
    the following.

    We proceed by distinguishing cases.

    \textit{Case 1.} Suppose first that $l = l'$. We distinguish
    subcases. 

 \textit{Subcase 1.1.} Suppose first that $l = l' = 1$. Then,
    \begin{align*}
      m_\Gamma &- m_{\Gamma'} ={}&\\ 
      &b \cdot \max\set{a_1^\Gamma, 1 + n_1^\Gamma} - b \cdot \max\set{a_1^{\Gamma'}, 1 + n_1^{\Gamma'}} \\
     ={}& ba_1^\Gamma - ba_1^{\Gamma'} \\
     ={}& ba_1^\Gamma - b(a_1^\Gamma + k_i - 1) = 0, \quad\text{since $k_i = 1$ by Claim~\ref{claim:levelsameandone}.}
    \end{align*}
    Hence, $m_{\Gamma'} \leq m_{\Gamma}$.

    \textit{Subcase 1.2.} Suppose that $l > 1$. Then one can verify that
    \begin{align*}
      m_\Gamma &- m_{\Gamma'} ={}&\\
      & b\cdot \max\set{a_l^\Gamma, 1 + n_l^\Gamma} + b \cdot \max\set{a_{l-1}^\Gamma, 1 + n_{l-1}^\Gamma} \\
      & - b \cdot \max\set{a_l^{\Gamma'}, 1 + n_l^{\Gamma'}} - b \cdot \max\set{a_{l-1}^{\Gamma'}, 1 + n_{l - 1}^{\Gamma'}}.
    \end{align*}

    Notice that, by Claim~\ref{claim:levelsame}, we know that
    $a_{l - 1}^{\Gamma'} \leq a_{l-1}^\Gamma + 1$. Now if
    $a_{l - 1}^{\Gamma'} = a_{l-1}^\Gamma$, we immediately obtain that
    $m_\Gamma - m_{\Gamma'} \geq 0$ by observing that
    $a_l^{\Gamma} = a_l^{\Gamma'}$ in this case. 

    Therefore, assume now that
    $a_{l - 1}^{\Gamma'} = a_{l-1}^\Gamma + 1$ also observe that we must
    have $n^{\Gamma'}_{l-1} = a_{l-1}^{\Gamma'}$ and
    $a_{l-1}^\Gamma = n_{l-1}^\Gamma$, since $\Gamma$ and $\Gamma'$ do
    not have any conflict-free atoms of level $l - 1$ by
    assumption. Moreover, notice that $n_l^{\Gamma'} = n_l^{\Gamma}$.

    From this bulk of information, we obtain
    \begin{align*}
      m_\Gamma &- m_{\Gamma'} ={}&\\
      & b\cdot {\max\set{a_l^{\Gamma'} + k_i, 1 + n_l^{\Gamma'}}} + b \cdot \max\set{a_{l-1}^{\Gamma'} -1,  a_{l-1}^{\Gamma'}} \\
               & - b \cdot \underbrace{\max\set{a_l^{\Gamma'}, 1 + n_l^{\Gamma'}}}_{=\, a_l^{\Gamma'} \text{ by Claim~\ref{claim:levelsucc}}} -\ b \cdot \max\set{a_{l-1}^{\Gamma'}, 1 + a_{l - 1}^{\Gamma'}} \\
      ={}& b  (a_l^{\Gamma'} + k_i) + b\cdot a_{l-1}^{\Gamma'} - b (a_{l-1}^{\Gamma'} - 1) - b\cdot a_l^{\Gamma'}\\
      ={}& b  (k_i - 1) \geq 0.
    \end{align*}
    This proves the claim for the case where $l = l' > 1$.    

    \textit{Case 2.} Now suppose that $l' = l - 1$. Observe that
    \begin{align*}
      m_{\Gamma} &- m_{\Gamma'} ={}& \\
                 & \sum_{i = 1}^{\lvl{\Sigma}} b \cdot \max\set{a_i^\Gamma, 1 + n_i^\Gamma} - \sum_{i = 1}^{\lvl{\Sigma}} b \cdot \max\set{a_i^{\Gamma'}, 1 + n_i^{\Gamma'}}  \\
      ={}& b \cdot \max\set{a_{l'}^{\Gamma}, 1 + n_{l'}^{\Gamma}} - b\cdot \max\set{a_{l'}^{\Gamma'}, 1 + n_{l'}^{\Gamma'}}\ + \\
                 & b \cdot \underbrace{\max\set{a_l^\Gamma, 1 + n_l^\Gamma}}_{=\, a_l^\Gamma \text{ by assumption}} -\ b \cdot \max\set{a_l^{\Gamma'}, 1 + n_l^{\Gamma'}} \\
       \geq{}&  b \cdot \max\set{a_{l'}^{\Gamma}, 1 + n_{l'}^{\Gamma}} - b\cdot \max\set{a_{l'}^{\Gamma'}, 1 + n_{l'}^{\Gamma'}},
    \end{align*}
    where the last inequality holds since
    $a_l^{\Gamma'} \leq a_l^\Gamma$ by piece-wise linearity and thus
    $\max\set{a_l^{\Gamma'}, 1 + n_l^{\Gamma'}} =
    \max\set{a_l^{\Gamma'}, 1 + n_l^{\Gamma}} \leq a_l^{\Gamma}$.
    
    By construction of $\Gamma'$, we know that
    $a_{l'}^\Gamma = n_{l'}^\Gamma$ and that
    $a_{l'}^{\Gamma'} \leq a^{\Gamma}_{l'} + k_i \leq a^{\Gamma}_{l'} +
    b$.

    We are going to distinguish two subcases. 

    \textit{Subcase 2.1.} Suppose first that
    $\max\set{a_{l'}^{\Gamma'}, 1 + n_{l'}^{\Gamma'}} =
    a_{l'}^{\Gamma'}$. Then,
    \begin{align*}
      m_\Gamma - m_{\Gamma'} = b (1 + n_{l'}^{\Gamma}) - b \cdot  a_{l'}^{\Gamma'} \geq 0,
    \end{align*}
    since $a_{l'}^{\Gamma'} \leq a_{l'}^\Gamma + b$ and
    $n_{l'}^\Gamma = a_{l'}^\Gamma$.

    \textit{Subcase 2.2.}  Suppose now that
    $\max\set{a_{l'}^{\Gamma'}, 1 + n_{l'}^{\Gamma'}} = 1 +
    n_{l'}^{\Gamma'}$.
    Now $1 + n_{l'}^{\Gamma'} \geq a_{l'}^{\Gamma'}$ entails that the
    number of conflict-free atoms in $\Gamma'[\ca{S}_{l'}]$ ist at most
    $1$. Since $l' = l - 1$, it must actually be the case that the
    number of conflict-free atoms in $\Gamma'[\ca{S}_{l'}]$ is exactly
    one, i.e., $a_{l'}^{\Gamma'} - n_{l'}^{\Gamma'} = 1$. Therefore, we
    must have $n_{l'}^{\Gamma'} = n_{l'}^{\Gamma}$. Now we obtain
    \begin{align*}
      m_\Gamma - m_{\Gamma'} = b(1 + n_{l'}^\Gamma) - b(1 + n_{l'}^{\Gamma'}) = 0,
    \end{align*}
    which proves that $m_\Gamma \geq m_{\Gamma'}$.
  \end{proof}

  By construction we know that $\ldpth{\Gamma_k} \leq n$, whence by
  induction hypothesis it follows that there is a reduction sequence
  $\pi' = \tup{\Gamma_{0,k},\Gamma_{1,k},\ldots,\Gamma_{k',k}, \Xi}$ for
  $\Gamma_k$ such that $\Gamma_{0,k} = \Gamma_k$,
  $\rk{\Gamma_{k',k}} \leq m$, and
  $m_{\Gamma_{0,k}} \geq m_{\Gamma_{1,k}} \geq \cdots \geq
  m_{\Gamma_{k',k}}$. Now we construct the reduction sequence
  \begin{align*}
    \pi \coloneqq \tup{\Gamma_0, \Gamma_1,\ldots,\Gamma_k, \Gamma_{1,k},\ldots,\Gamma_{k',k}, \Xi},
  \end{align*}
  and recall that $\Gamma_0 = \Gamma$. Now Claim~\ref{claim:main-claim-pwl} yields
  $m_\Gamma = m_{\Gamma_0} \geq m_{\Gamma_1} \geq \cdots \geq
  m_{\Gamma_k}$,
  whence it follows that
  \begin{align*}
    m_\Gamma = m_{\Gamma_0} \geq m_{\Gamma_1} \geq \cdots \geq
  m_{\Gamma_k} \geq m_{\Gamma_{1,k}} \geq \cdots \geq m_{\Gamma_{k',k}}.
  \end{align*}
  Thus, $\pi$ is a reduction sequence for $\Gamma$. This concludes the
  induction step of our subsidiary induction on $\ldpth{\Gamma}$ and
  thus the proof of Lemma~\ref{lem:redsequence}.
  \end{proof}

  We can now easily conclude the induction step for the induction on
  $\rk{\Gamma}$ as follows. We know by Lemma~\ref{lem:redsequence} that
  there is a reduction sequence
  $\tup{\Gamma_0,\Gamma_1,\ldots,\Gamma_k,\Xi}$ for $\Gamma$ such that
  \begin{enumerate}
  \item $\Gamma_0 = \Gamma$, 
  \item $m_{\Gamma_0} \geq m_{\Gamma_1} \geq \cdots \geq m_{\Gamma_k}$,
  \item each $\Gamma_{i+1}$ is an unfolding of $\Gamma_i$, where
    $i = 0,\ldots,k-2$,
  \item $\rk{\Gamma_k} \leq m$, and
  \item $\Xi = \Gamma_{k-1} \cap D$ and
    $\Gamma_{k} = \Gamma_{k-1} \setminus \Xi$.
  \end{enumerate}
   Now since
  $\rk{\Gamma_k} \leq m$, by induction hypothesis, there exists a linear
  chase tree $\ca{T}'$ for $\Gamma_k$ whose node-width is bounded by
  $m_{\Gamma_k}$. Let $\ca{T}$ be the linear chase tree for $\Gamma$
  constructed as follows. The root $v_0$ of $\ca{T}$ is labeled
  $\Gamma$, and there are nodes $v_1,\ldots,v_k, v_k'$ such that
  \begin{enumerate*}[label={(\roman*)}]
  \item for all $i = 0,1,\ldots,k - 1$, $v_i$ is labeled with $\Gamma_i$,
  \item $v_{i+1}$ is the only child of $v_i$, for all $i = 0,1,\ldots,k-2$, while
  \item $v_{k-1}$ has two children, namely $v_k$ and $v_k'$, where the
    former is labeled with $\Gamma_k$, and the latter is labeled with
    $\Xi$.
  \end{enumerate*}
  We declare that $\ca{T}'$ is a subtree of $\ca{T}$ that is rooted in
  $v_k$. Then $\ca{T}$ is a linear chase tree for $\Gamma$ whose
  node-width is bounded by $m_\Gamma$, as required. This concludes the
  induction step and thus the proof of item (2) of
  Lemma~\ref{lem:existence-ct}.
\end{proof}

\subsection{Proof of Lemma~\ref{lem:from-ct-to-pt}}

Recall that $D$ is a database and $\Sigma$ a set of TGDs. Consider the
chase graph $\ca{G}^{D,\Sigma}$ for $D$ and $\Sigma$, and the unraveling
$\ca{G}^{D,\Sigma}_\Theta$ of $\ca{G}^{D,\Sigma}$ around some
$\Theta \subseteq \chase{D}{\Sigma}$. Suppose $p(\ve{x})$ is a CQ with
$\ve{x} = x_1,\ldots,x_n$, and suppose $h$ is a homomorphism such that
$h(\atoms{p}) \subseteq U(\ca{G}^{D,\Sigma},\Theta)$.

For a sequence of variables $\ve{v}$ that are all among $\var{q}$, we
let $\sim_{h,\ve{v}}$ be the equivalence relation defined by
$$v_i \sim_{h,\ve{v}} v_j \iff h(v_i) = h(v_j),$$
and we let $\pi_{h,\ve{v}}$ be the partition of the variables
$\ve{v}$ given by the set of equivalence classes of $\sim_{h,\ve{v}}$.

We show the following lemma which is a slightly more general statement
than that of Lemma~\ref{lem:from-ct-to-pt}:

\begin{lemma}
  \label{lem:ptct}
  If there is a (linear) chase tree $\ca{T}$ for $h(\atoms{p})$
  w.r.t.~$\ca{G}^{D,\Sigma}_\Gamma$ such that $\nwd{\ca{T}} \leq m$, then
  there is a (linear) proof tree $\ca{P}$ of $p(\ve{x})$ w.r.t.~$\Sigma$
  such that
  \begin{enumerate}
  \item $\ca{P}$ has equality type $\pi_{h,\ve{x}}$,
  \item $\nwd{\ca{P}} \leq m$, and
  \item$\ve{c} \in p_{\ca{P}}(D)$.
  \end{enumerate}
\end{lemma}
\begin{proof}
  Let $\alpha_1,\ldots,\alpha_s$ be an enumeration of the body atoms of
  $p(\ve{x})$. We proceed by induction on the depth of $\ca{T}$ (i.e.,
  the longest among all paths that lead from the root to a leaf).

  Suppose first that the depth of $\ca{T}$ equals $1$, that is, $\ca{T}$
  consists of just a single node $v_0$ whose label equals $h(\atoms{p})$. Then
  the proof tree $\ca{P}$ that just consists of a single node labeled
  with
  \begin{align*}
    P(\eq_{\pi_{h,\ve{x}}}(x_1,\ldots,x_n)) \la \eq_{\pi_{h,\ve{x}}}(\alpha_1,\ldots,\alpha_s),
  \end{align*}
  is obviously a proof tree for $p(\ve{x})$ w.r.t.~$\Sigma$ such that
  $\ve{c} \in p_{\ca{P}}(D)$.

  Suppose now that the depth of $\ca{T}$ is larger than one such that
  $\nwd{\ca{T}} \leq m$. We distinguish cases.

  \textit{Case 1.} Suppose first that the children of the root $v_0$ of
  $\ca{T}$ -- whose label equals $h(\atoms{p})$ -- result from a decomposition
  step. Assume that $v_0$ has exactly two children, say $v_1$ and $v_2$,
  that are respectively labeled $\Theta_1$ and $\Theta_2$ -- the case
  with any other number of children is treated analogously. Therefore,
  $\set{\Theta_1,\Theta_2}$ must be a decomposition of $h(\atoms{p})$ such that
  $h(\atoms{p}) = \Theta_1 \cup \Theta_2$, and $\Theta_1$ and $\Theta_2$ do not
  share any labeled null. Let $\ca{T}_1$ and $\ca{T}_2$ respectively be
  the subtrees rooted in $v_1$ and $v_2$, and notice that
  $\nwd{\ca{T}_1} \leq m$ and $\nwd{\ca{T}_2} \leq m$. Moreover, let
  $\ve{y} = y_1,\ldots,y_k$ be the list of variables from
  $\var{p} \setminus \set{x_1,\ldots,x_n}$ such that $h(y_i)$ is a
  constant, and $y_i$ occurs in atoms $\alpha$ and $\beta$ of
  $p(\ve{x})$, but neither $h(\set{\alpha,\beta}) \subseteq \Theta_1$,
  nor $h(\set{\alpha,\beta}) \subseteq \Theta_2$ holds.

  Let $\ca{P}$ be the proof tree whose root $v_0$ is labeled with
  \begin{align}
    P(\eq_{\pi_{h,\ve{x}}}(\ve{x})) \la \eq_{\pi_{h,\ve{x}}}(\alpha_1,\ldots,\alpha_s),
  \end{align}
  and that has exactly one child $v'$ whose label is
  \begin{align}
    P'(\eq_{\pi_{h,\ve{x},\ve{y}}}(\ve{x},\ve{y})) \la \eq_{\pi_{h,\ve{x},\ve{y}}}(\alpha_1,\ldots,\alpha_s).
  \end{align}
  It is easy to check that (2) results from a specialization step
  from (1). Now let $\beta_{i_1},\ldots,\beta_{i_l}$ be those atoms from
  $\eq_{\pi_{h,\ve{x},\ve{y}}}(\alpha_1,\ldots,\alpha_s)$ whose image
  under $h$ lies in $\Theta_1$, and $\beta_{j_1},\ldots,\beta_{j_r}$
  those whose image under $h$ lies in $\Theta_2$. Let $\ve{z}$ be the
  restriction of $\eq_{\pi_{h,\ve{x},\ve{y}}}(\ve{x},\ve{y})$ to
  $\var{\set{\beta_{i_1},\ldots,\beta_{i_l}}}$, and let $\ve{w}$ be the
  restriction of $\eq_{\pi_{h,\ve{x},\ve{y}}}(\ve{x},\ve{y})$ to
  $\var{\set{\beta_{j_1},\ldots,\beta_{j_r}}}$. We let $v_1$ and $v_2$
  be children of $v'$ in $\ca{P}$ whose labels are respectively
  $P_1(\ve{z}) \la \beta_{i_1},\ldots,\beta_{i_l}$ and
  $P_2(\ve{w}) \la \beta_{j_1},\ldots,\beta_{j_r}$. Then these two
  queries result from a decomposition step from (2). Since
  $h(\set{\beta_{i_1},\ldots,\beta_{i_l}}) = \Theta_1$ and
  $h(\set{\beta_{j_1},\ldots,\beta_{j_r}}) = \Theta_2$, by induction
  hypothesis, there are proof trees $\ca{P}_1$ and $\ca{P}_2$ that have
  equality types $\pi_{h, \ve{z}}$ and $\pi_{h,\ve{w}}$, respectively,
  such that $\nwd{\ca{P}_1} \leq m$ and $\nwd{\ca{P}_2} \leq m$.
  Furthermore, we have $h(\ve{z}) \in p_{\ca{P}_1}(D)$ and
  $h(\ve{w}) \in p_{\ca{P}_2}(D)$. Notice that
  $\eq_{\pi_{h, \ve{z}}}(\ve{z}) = \ve{z}$ and
  $\eq_{\pi_{h, \ve{w}}}(\ve{w}) = \ve{w}$ by construction. Moreover,
  $\exists\ve{v}\, (p_{\ca{P}_1}(\ve{z}) \land p_{\ca{P}_2}(\ve{w}))
  \equiv p_{\ca{P}}$, where $\ve{v}$ is the sequence of variables that
  appear in the head of (2), but not in the head of (1). Hence,
  $\ve{c} \in p_{\ca{P}}(D)$ and $\ca{P}$ is thus the proof tree of
  $p(\ve{x})$ w.r.t.~$\Sigma$ we are looking for.

  \textit{Case 2.} Suppose now that the root $v_0$ of $\ca{T}$ has
  exactly one child, say $v'$, that is labeled with $\Theta'$ which
  results from $h(\atoms{p})$ by unfolding. Let $\sigma \in \Sigma$, $h_0$,
  $\beta_1,\ldots,\beta_k$, and $\alpha \in h(\atoms{p})$ be such that
  $\preds{\alpha}{\sigma}{h_0} = \set{\beta_1,\ldots,\beta_k}$ and
  $\Theta' = (h(\atoms{p}) \setminus \set{\alpha}) \cup
  \set{\beta_1,\ldots,\beta_k}$. Thus, $\sigma$ is of the form
  \begin{align*}
    p_{\beta_1}(\ve{x}_1),\ldots,p_{\beta_k}(\ve{x}_k) \limpl \exists w_{i_1},\ldots,w_{i_l}\, p_{\alpha}(w_1,\ldots,w_r),
  \end{align*}
  for some predicates $p_{\beta_1},\ldots,p_{\beta_k},\alpha$.
  Moreover, $p(\ve{x})$ contains an atom of the form
  $p_\alpha(t_1,\ldots,t_r)$ such that
  $$h(p_\alpha(t_1,\ldots,t_r)) = \alpha = h_0(p_\alpha(w_1,\ldots,w_r))$$
  (the $t_1,\ldots,t_r$ are terms each of which is either a variable or
  a constant).  Now let $\sigma_{v_0}$ be a copy of $\sigma$, where
  every variable occurrence $x$ is renamed to $x_{v_0}$. Let $h'$ be the
  homomorphism defined by $h'(x_{v_0}) \coloneqq h_0(x)$. Moreover, let
  $\eq_{\pi_{h,\ve{x}}}(t_1,\ldots,t_r) = s_1,\ldots,s_r$. Notice that
  $\set{t_1,\ldots,t_r} \subseteq \set{s_1,\ldots,s_r}$ and observe that
  $h(p_\alpha(s_1,\ldots,s_r)) = \alpha =
  h'(p_\alpha(w_{1,v_0},\ldots,w_{r,v_0}))$.  Let $\gamma$ be a
  substitution such that, for all $i, j \in [r]$,
  \begin{align*}
  \gamma(z_i) = \gamma(w_{j,v_0}) \coloneqq v_t \iff  t = h(z_i) = h'(w_{j,v_0}),
  \end{align*}
  where the $v_t$ are newly chosen variable names (for the other
  variables not mentioned, $\gamma$ is simply the identity).  In
  particular, $\gamma(x_i) = \gamma(x_j)$ iff $x_i \sim_{h,\ve{x}} x_j$,
  for all output variables $x_i$ and $x_j$ of $p(x_1,\ldots,x_n)$ that
  are among $\set{s_1,\ldots,s_r}$. Let $\gamma_0$ be an MGU such that
  $\gamma = \eta \circ \gamma_0$ for some substitution $\eta$. Notice
  that, if $x_i$ and $x_j$ are output variables of $p(\ve{x})$ among
  $\set{s_1,\ldots,s_r}$, then $\gamma_0(x_i) = \gamma_0(x_j)$ implies
  $x_i \sim_{h,\ve{x}} x_j$. On the other hand -- writing
  $\hat{x}_1,\ldots,\hat{x}_{n}$ for the sequence
  $\eq_{\pi_{h,\ve{x}}}(x_1,\ldots,x_n)$ -- if $x_i \sim_{h,\ve{x}} x_j$,
  then there is exactly one $v \in \set{\hat{x}_1,\ldots,\hat{x}_n}$
  such that $h(v) = h(x_i) = h(x_j)$. Thus, $\gamma_0$ is bijective when
  restricted to the (representatives of the) equivalence classes of
  $\sim_{h,\ve{x}}$ and we can henceforth assume w.l.o.g.~that
  $\gamma_0(\hat{x}_i) = \hat{x}_i$ for all $i = 1,\ldots,{n}$.

  Let $\ca{P}$ be the proof tree with equality type $\pi_{h,\ve{x}}$
  whose root $v_0$ is labeled with
   \begin{align}
    P(\hat{x}_1,\ldots,\hat{x}_{{n}}) \la \eq_{\pi_{h,\ve{x}}}(\alpha_1,\ldots,\alpha_s).
  \end{align}
  We introduce a new node $v'$
  in $\ca{P}$ that is a child of $v_0$ and whose label is
  \begin{align}
    P'(\hat{x}_1,\ldots,\hat{x}_{{n}}) \la \gamma_0(A),
  \end{align}
  where
  \begin{align*}
    A \coloneqq{}& (\eq_{\pi_{h,\ve{x}}}(\set{\alpha_1,\ldots,\alpha_s}) \setminus \set{p_\alpha(s_1,\ldots,s_r)})\ \cup \\  &\set{p_{\beta_1}(\ve{x}_{1,v_0}),\ldots,p_{\beta_k}(\ve{x}_{k,v_0})}.
  \end{align*}
  It is clear that (4) is a $\sigma_{v_0}$-resolvent of (3). Notice in
  particular that the variables occurring in
  $\eq_{\pi_{h,\ve{x}}}(\alpha_1,\ldots,\alpha_s)$ and that unify with
  some existential variable from the head of $\sigma_{v_0}$ cannot be
  shared, since the application of
  $\beta_1,\ldots,\beta_k \Ra_{\sigma,h_0} \alpha$ is not blocked in
  $h(\atoms{p})$. Moreover, the resolvent must be IDO, since $\gamma_0$ is the
  identity on $\set{\hat{x}_1,\ldots,\hat{x}_{{n}}}$. 

  Let us write $p'(\hat{x}_1,\ldots,\hat{x}_n)$ for the CQ (4). Now let
  $h''$ be the homomorphism that extends $h$ so that $h''$ maps
  $p'$ to $\Theta'$ and
  $h''(\hat{x}_1,\ldots,\hat{x}_n) = \ve{c}$. Notice that $h''$ exists
  by construction. Now the subtree of $\ca{T}$ that is rooted at $v'$,
  call it $\ca{T}'$, has smaller depth than $\ca{T}$, whence by
  induction hypothesis it follows that there is a proof tree $\ca{P}'$
  of $p'$ w.r.t.~$\Sigma$ such that
  \begin{enumerate*}[label={(\roman*)}]
  \item $\ca{P}'$ has equality type
    $\pi_{h'',\hat{x}_1,\ldots,\hat{x}_n}$,
  \item $\nwd{\ca{P}'} \leq m$, and
  \item $\ve{c} \in p'_{\ca{P}'}(D)$.
  \end{enumerate*}
  We can thus simply declare that $\ca{P}'$ becomes a subtree of
  $\ca{P}$ rooted at the node $v'$ of $\ca{P}$. Then $\ca{P}$ is a proof
  tree for $p(x_1,\ldots,x_n)$ that has equality type $\pi_{h,\ve{x}}$
  and for which it holds that $\nwd{\ca{P}} \leq m$. Moreover, we must
  have $\ve{c} \in p_{\ca{P}}(D)$, since $\ca{P}$ and $\ca{P}'$ have the
  same leaf nodes. 

  Notice that the construction performed in the cases above yields a
  linear $\ca{P}$ whenever $\ca{T}$ is linear, and thus
  Lemma~\ref{lem:ptct} follows.
\end{proof}

%%% Local Variables:
%%% fill-column: 72
%%% TeX-PDF-mode: t
%%% TeX-debug-bad-boxes: t
%%% TeX-master: "main.tex"
%%% TeX-parse-self: t
%%% TeX-auto-save: t
%%% reftex-plug-into-AUCTeX: t
%%% End:
